# Supplementary material for: Rapid quantitative magnetization transfer imaging: utilizing the hybrid state and the generalized Bloch model
Source: arXiv:2207.08259 source file (2023-11-25)
Supplement: Supplementary file 3 [file SupportingInformation-figure4.pdf]

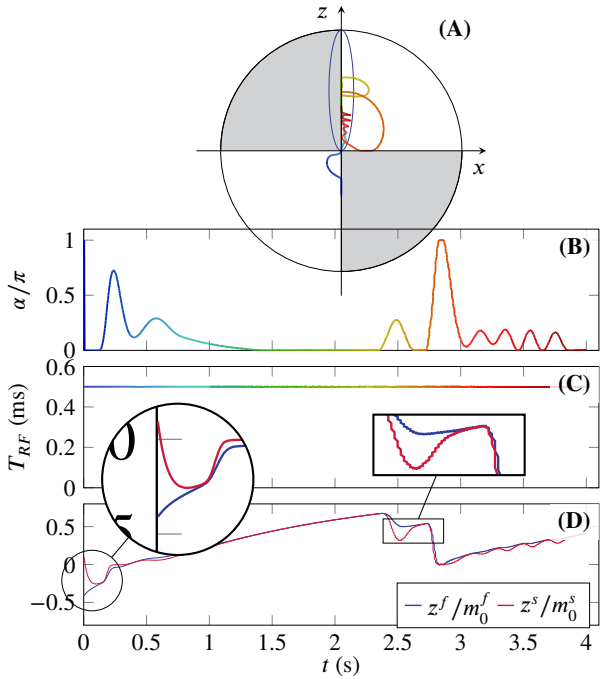

### **Temporary page!**

$\LaTeX$  was unable to guess the total number of pages correctly. As there was some unprocessed data that should have been added to the final page this extra page has been added to receive it.

If you rerun the document (without altering it) this surplus page will go away, because  $\LaTeX$  now knows how many pages to expect for this document.
